# Supplementary material for: CaBaFL: Asynchronous Federated Learning via Hierarchical Cache and Feature Balance
Source: arXiv:2404.12850 source file (2024-07-17)
Supplement: Supplementary file 1 [file appendix.tex]

\clearpage
\appendix

\section{Appendix}
% \section{Appendix}\label{sec:appendix}
\subsection{Experimental Results for Accuracy Comparison}
In this section, we present all the experimental results. Figures \ref{start}-\ref{end} compare learning curves between CaBaFL and all the baselines on three datasets with different non-IID and IID settings using ResNet-18, CNN, and VGG-16 models.

\begin{figure}[h]
\centering
\footnotesize
\subfloat[$\beta = 0.1$]{\includegraphics[width=0.45\columnwidth]{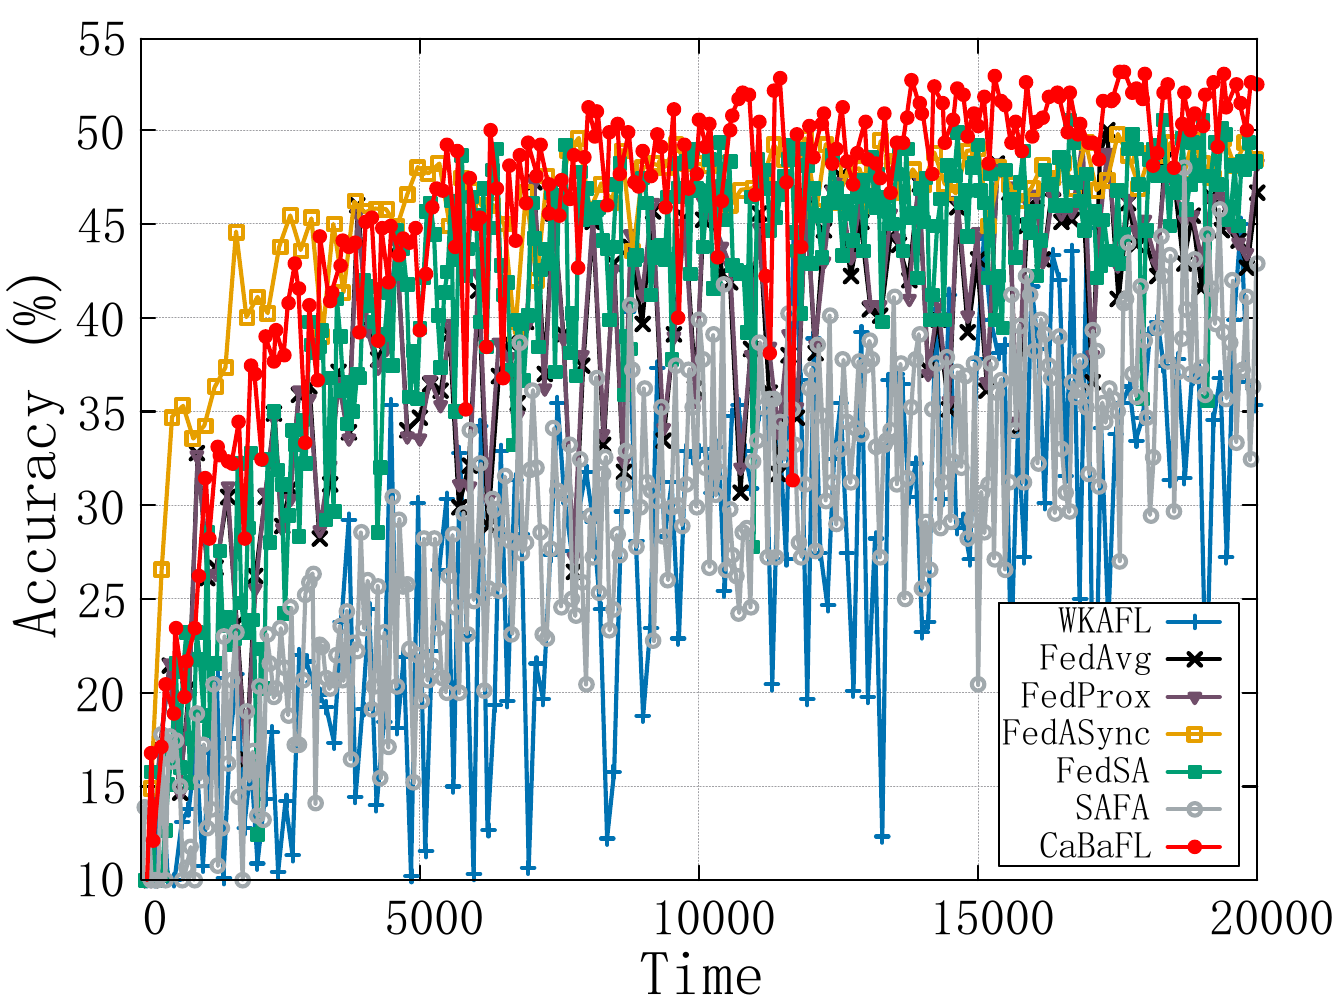}%
\label{fig:real_testbed}}
\hfil
\subfloat[$\beta = 0.5$]{\includegraphics[width=0.45\columnwidth]{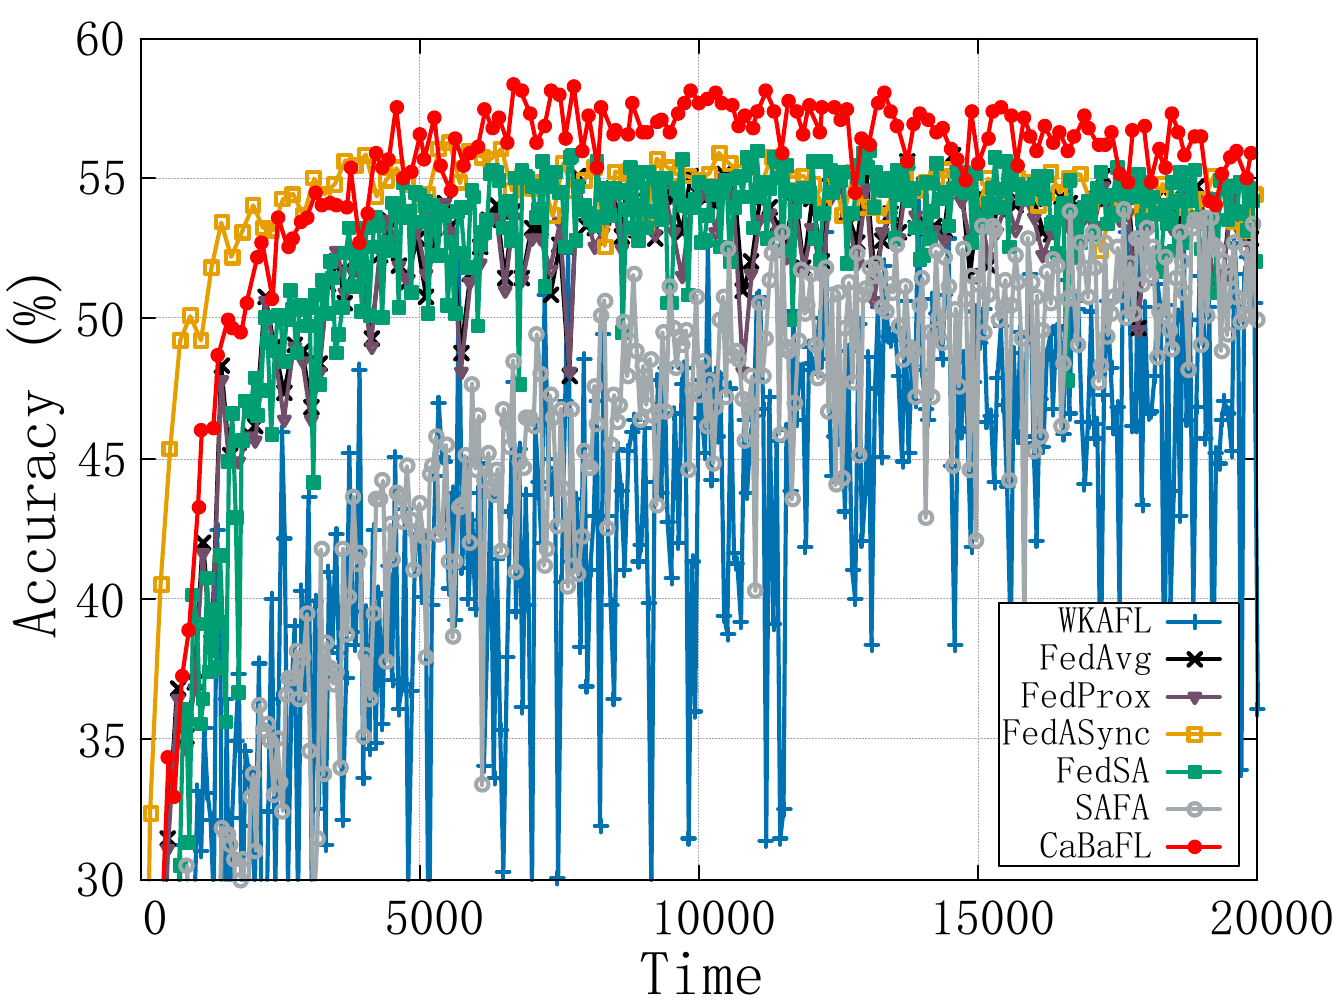}%
\label{fig:real-cifar-10-IID-ls}}
\hfil
\subfloat[$\beta = 1.0$]{\includegraphics[width=0.45\columnwidth]{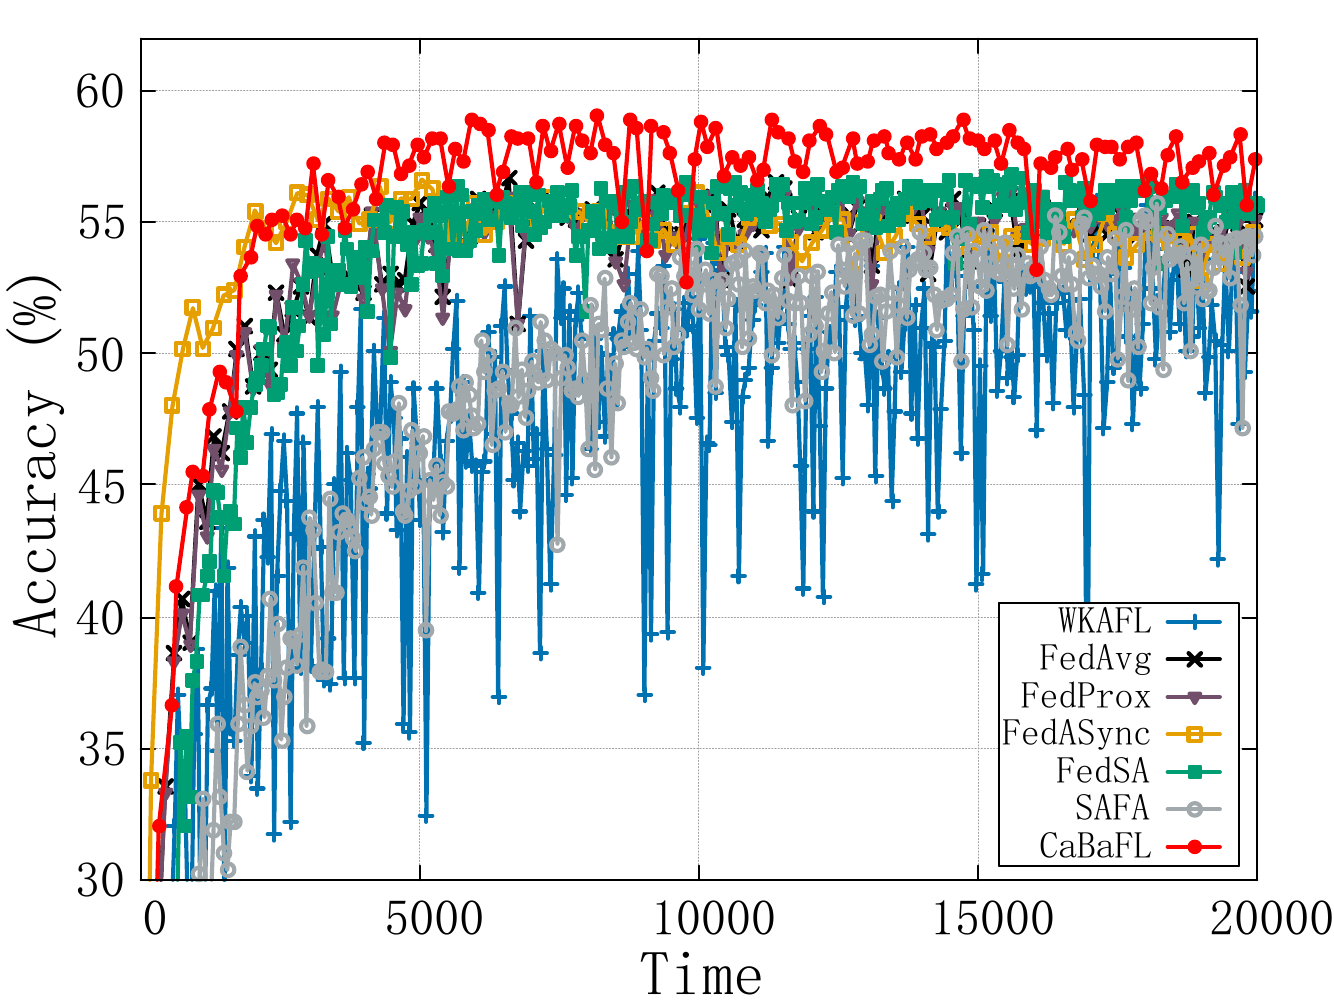}%
\label{fig:real-cifar-10-IID-lm}}
\hfil
\subfloat[IID]{\includegraphics[width=0.45\columnwidth]{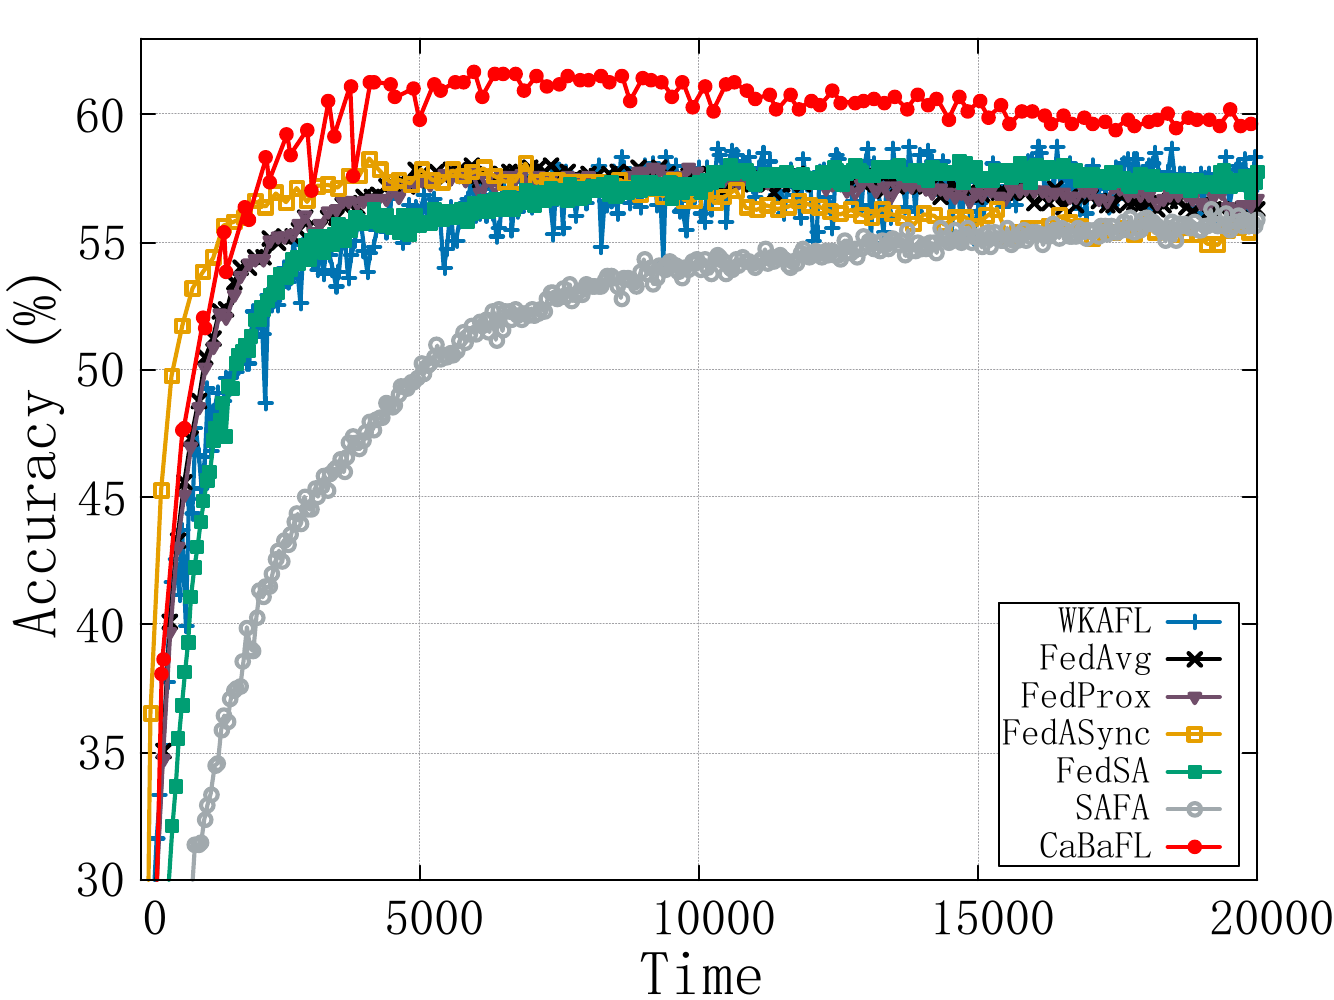}%
\label{fig:real_testbed}}
\caption{Learning curves of CaBaFL and all the baseline methods on CIFAR-10 and CNN.}
\label{start}
\end{figure}

\begin{figure}[h]
\centering
\footnotesize
\subfloat[$\beta = 0.1$]{\includegraphics[width=0.45\columnwidth]{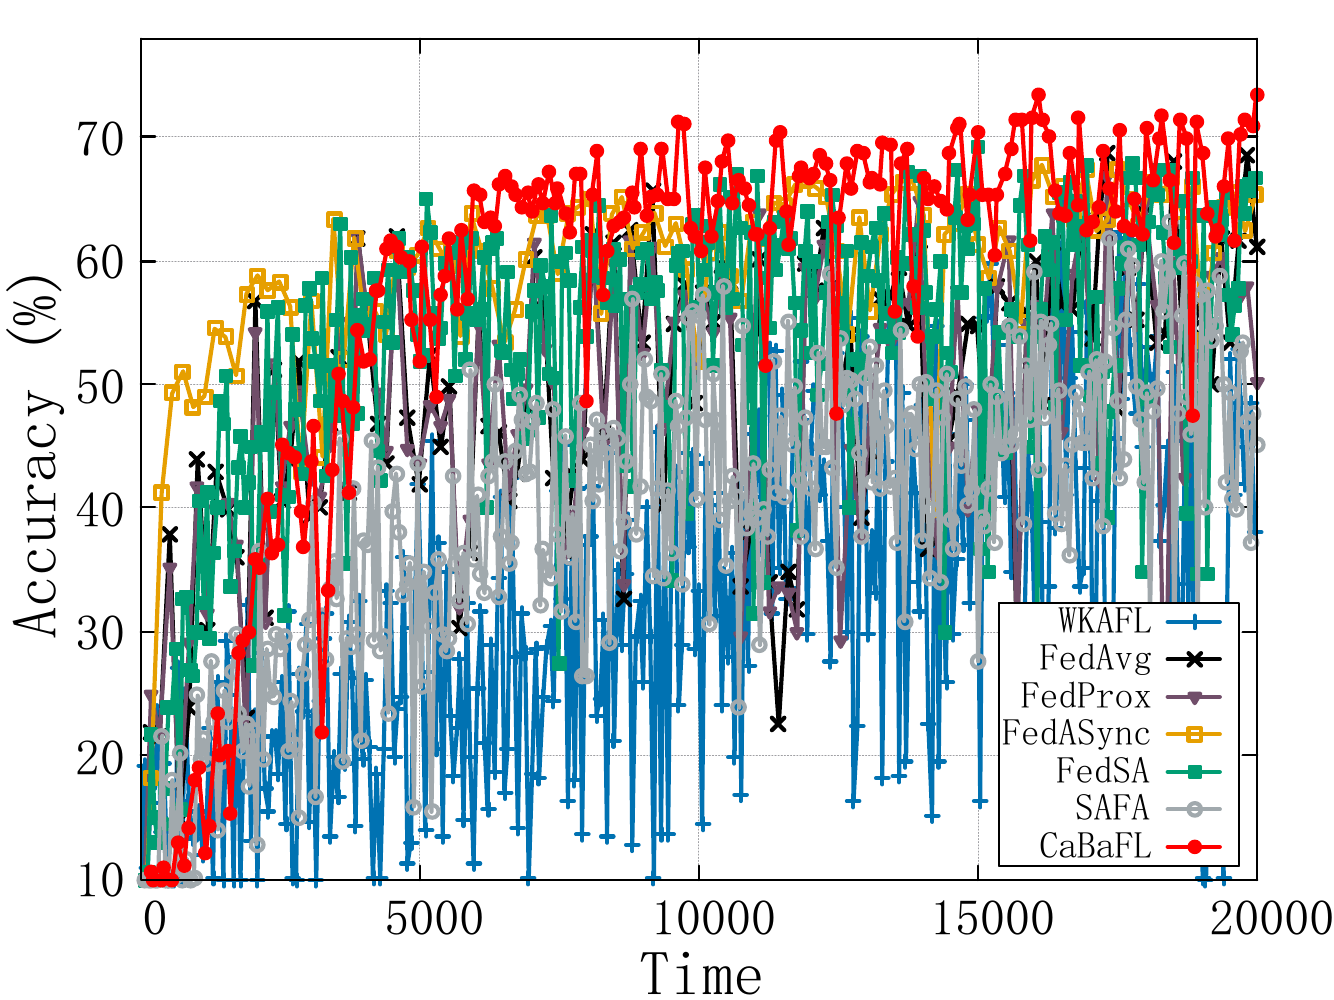}%
\label{}}
\hfil
\subfloat[$\beta = 0.5$]{\includegraphics[width=0.45\columnwidth]{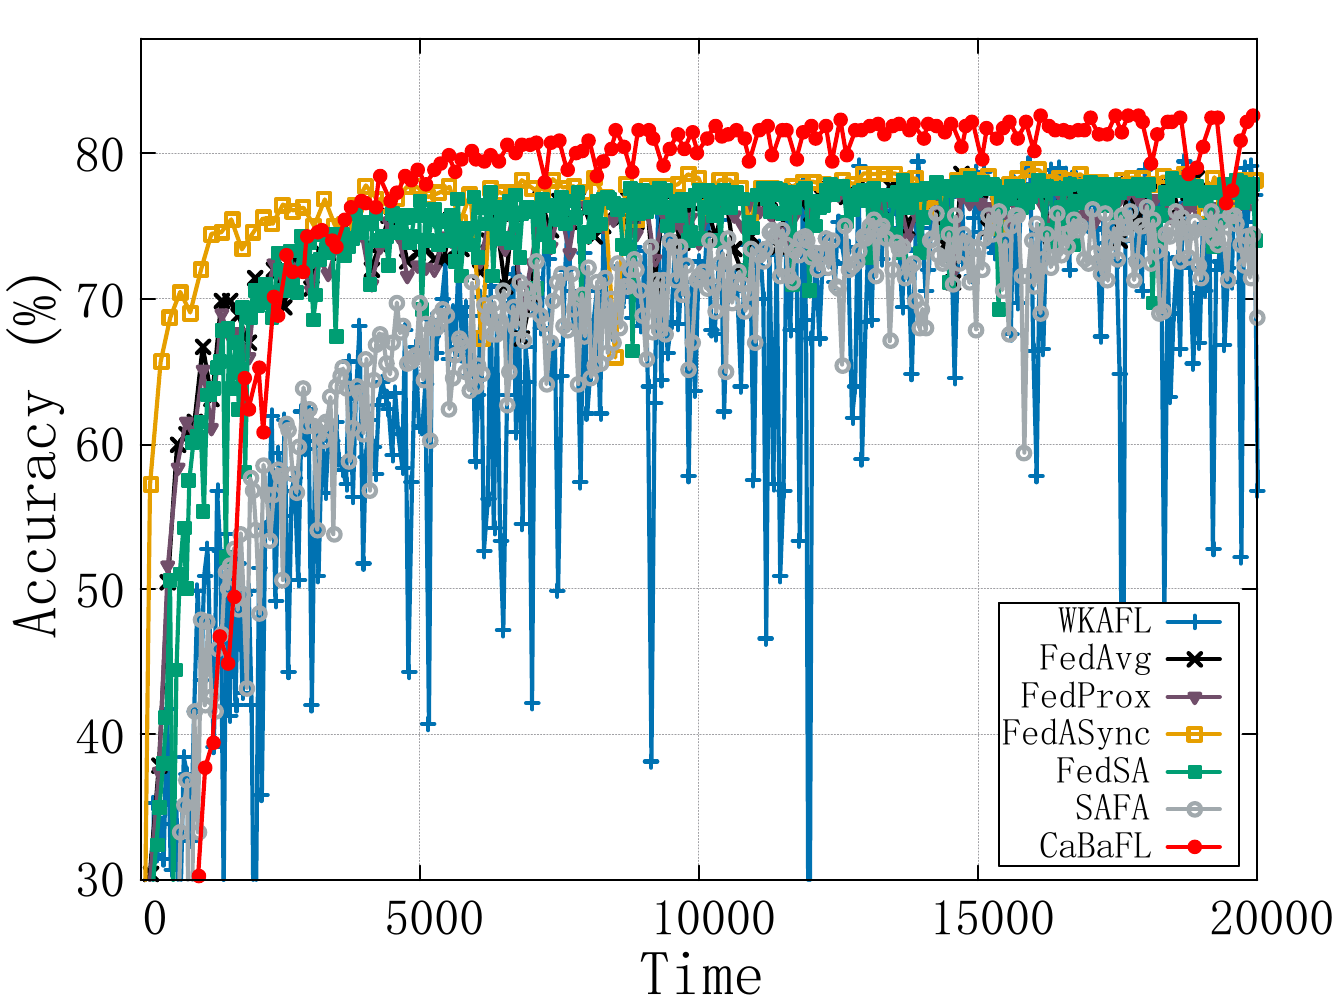}%
\label{}}
\hfil
\subfloat[$\beta = 1.0$]{\includegraphics[width=0.45\columnwidth]{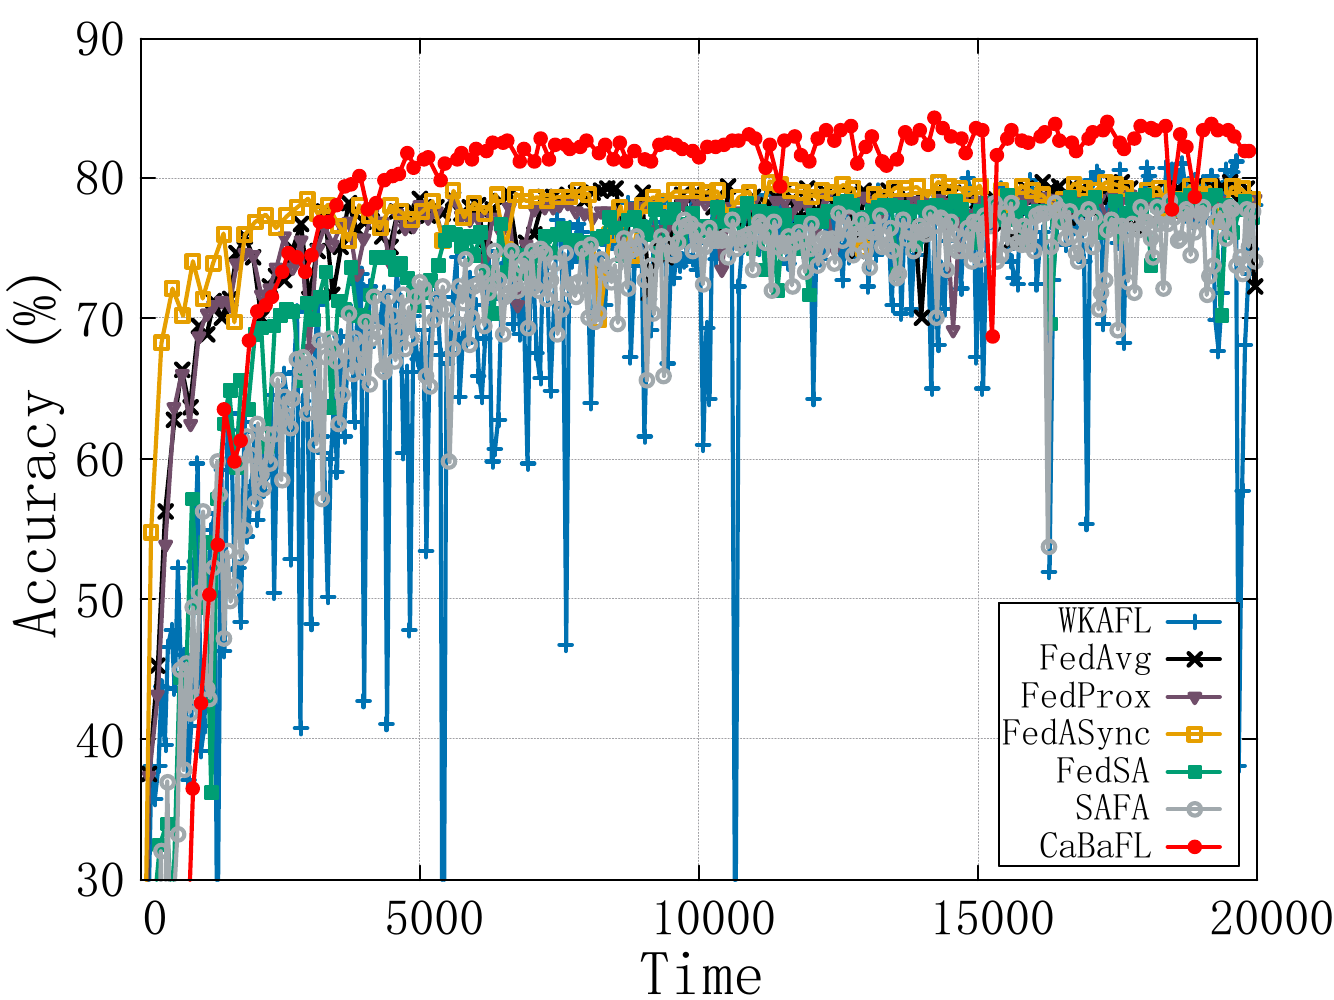}%
\label{}}
\hfil
\subfloat[IID]{\includegraphics[width=0.45\columnwidth]{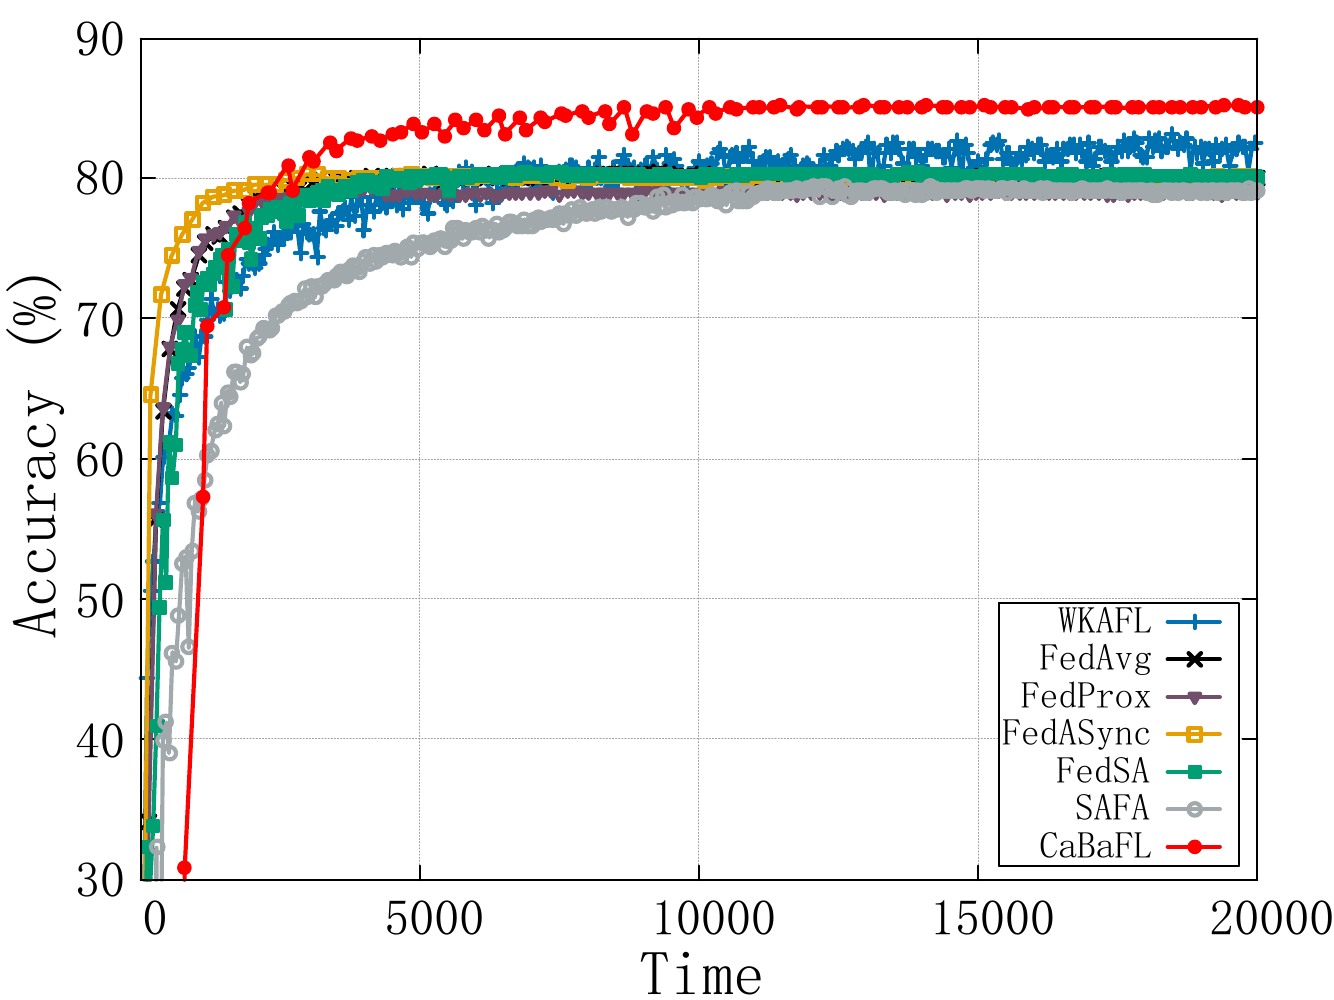}%
\label{}}
\caption{Learning curves of CaBaFL and all the baseline methods on CIFAR-10 and VGG-16.}
\end{figure}

\begin{figure}[h]
\centering
\footnotesize
\subfloat[$\beta = 0.1$]{\includegraphics[width=0.45\columnwidth]{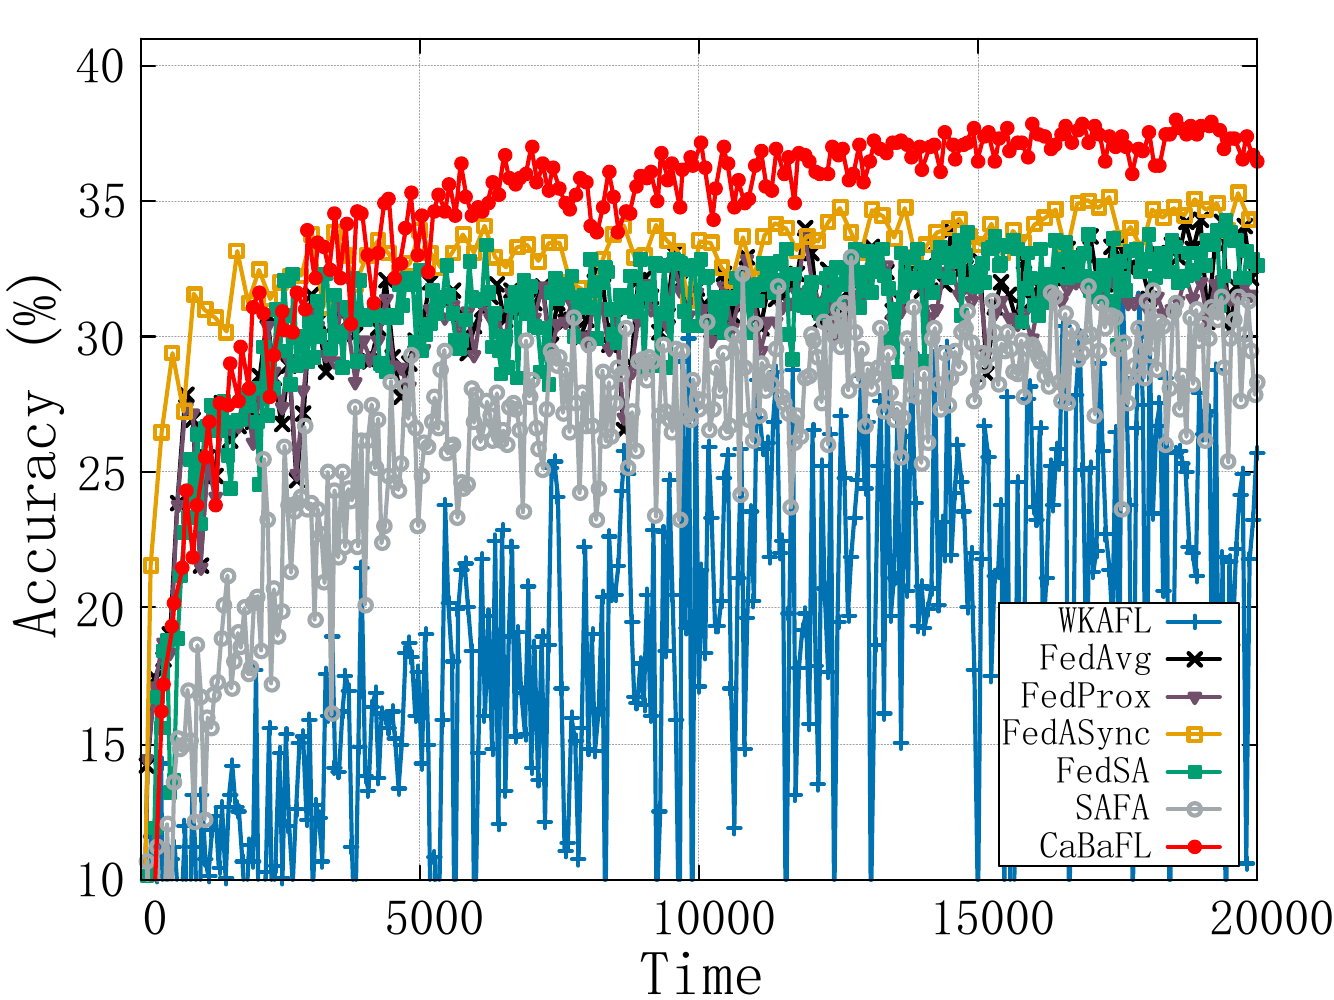}%
\label{}}
\hfil
\subfloat[$\beta = 0.5$]{\includegraphics[width=0.45\columnwidth]{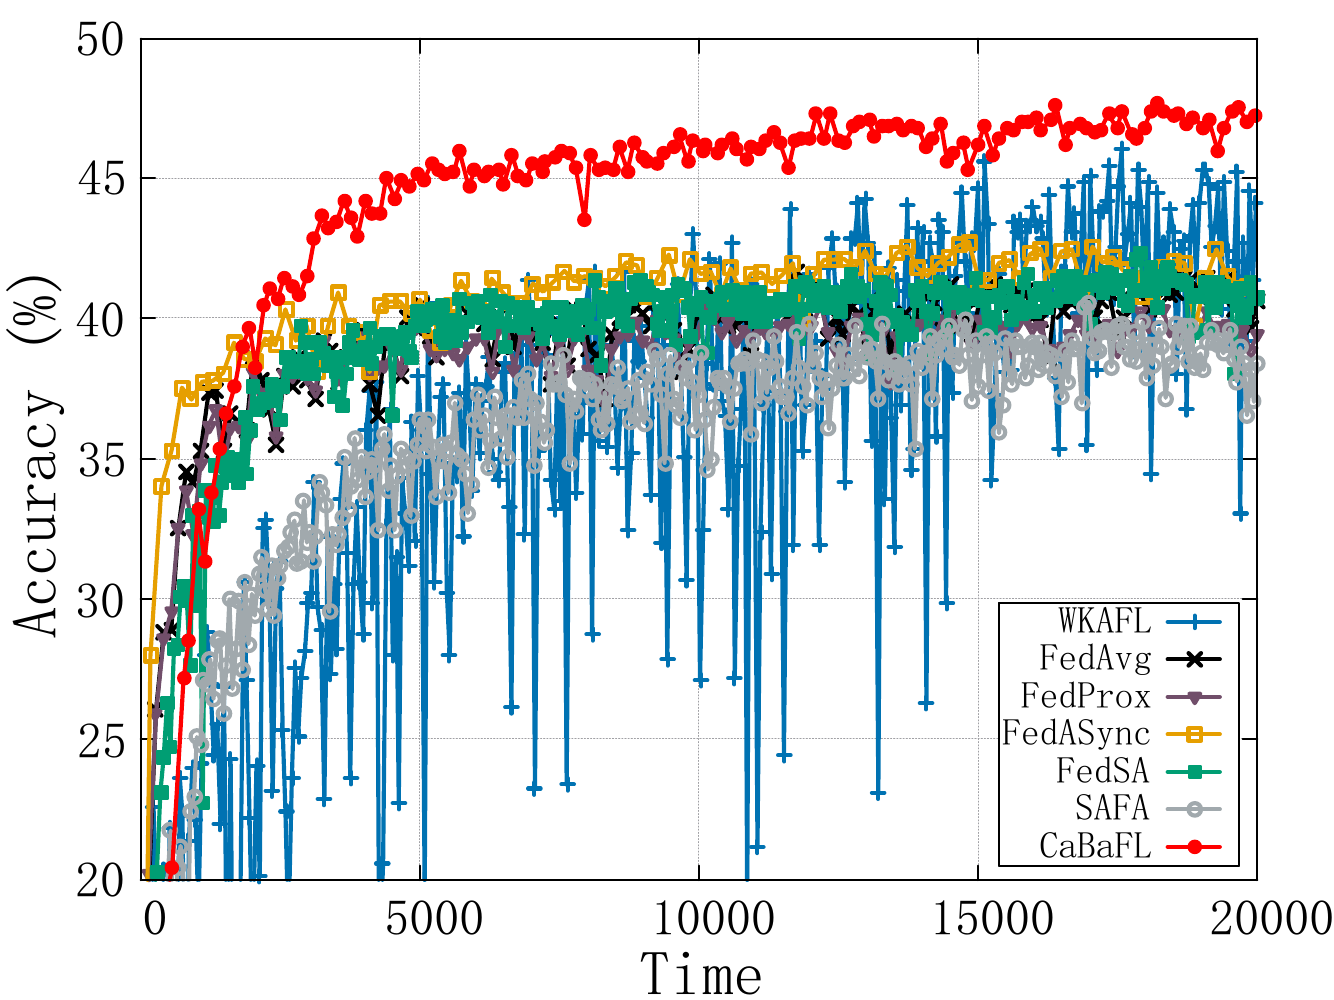}%
\label{}}
\hfil
\subfloat[$\beta = 1.0$]{\includegraphics[width=0.45\columnwidth]{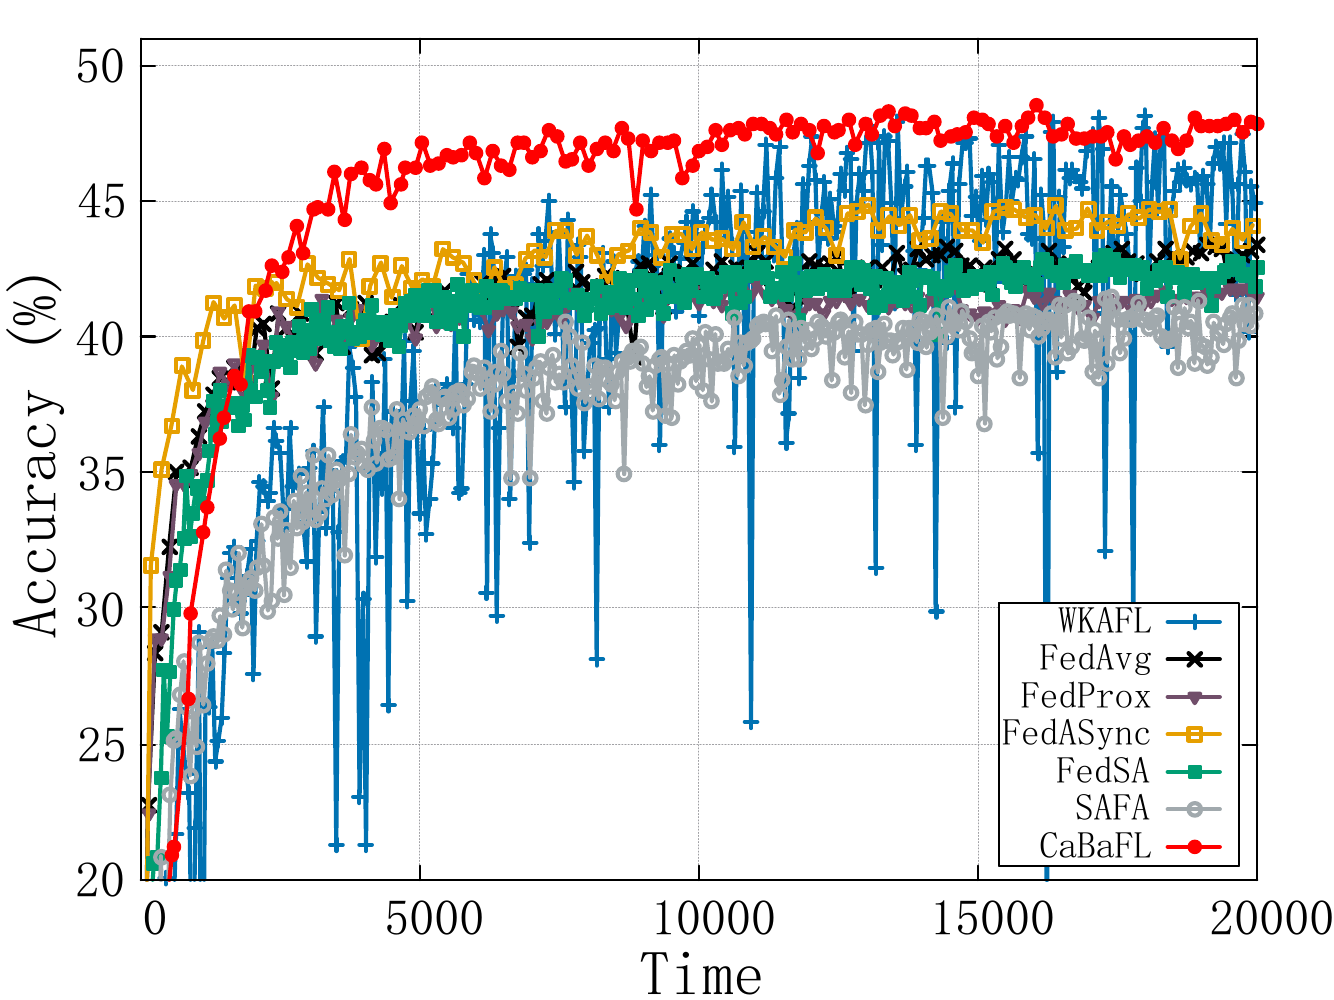}%
\label{}}
\hfil
\subfloat[IID]{\includegraphics[width=0.45\columnwidth]{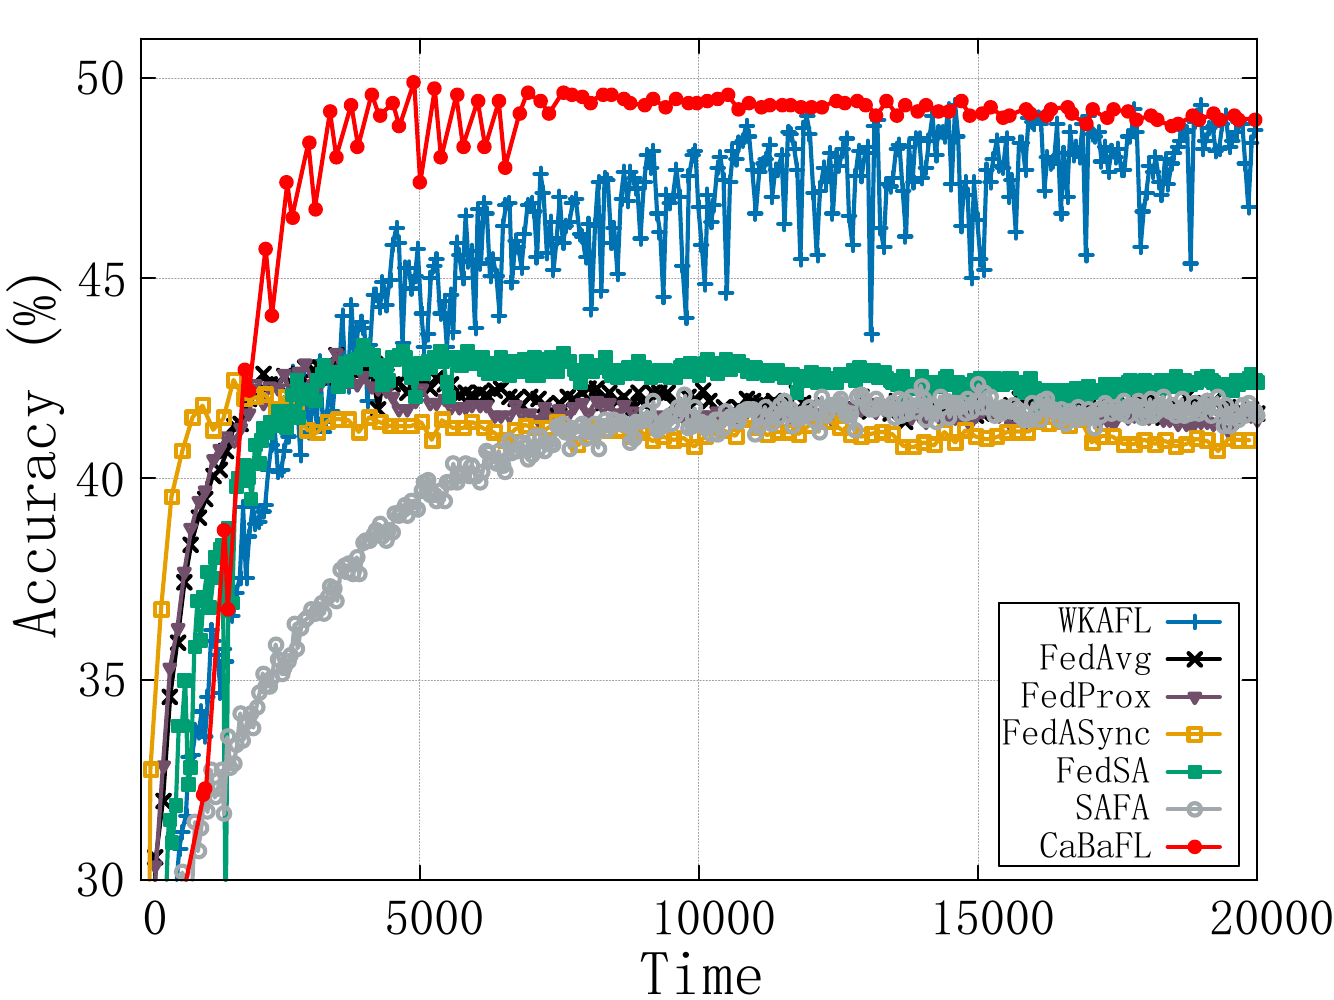}%
\label{}}
\caption{Learning curves of CaBaFL and all the baseline methods on CIFAR-100 and ResNet-18.}
\end{figure}

\begin{figure}[h]
\centering
\footnotesize
\subfloat[$\beta = 0.1$]{\includegraphics[width=0.45\columnwidth]{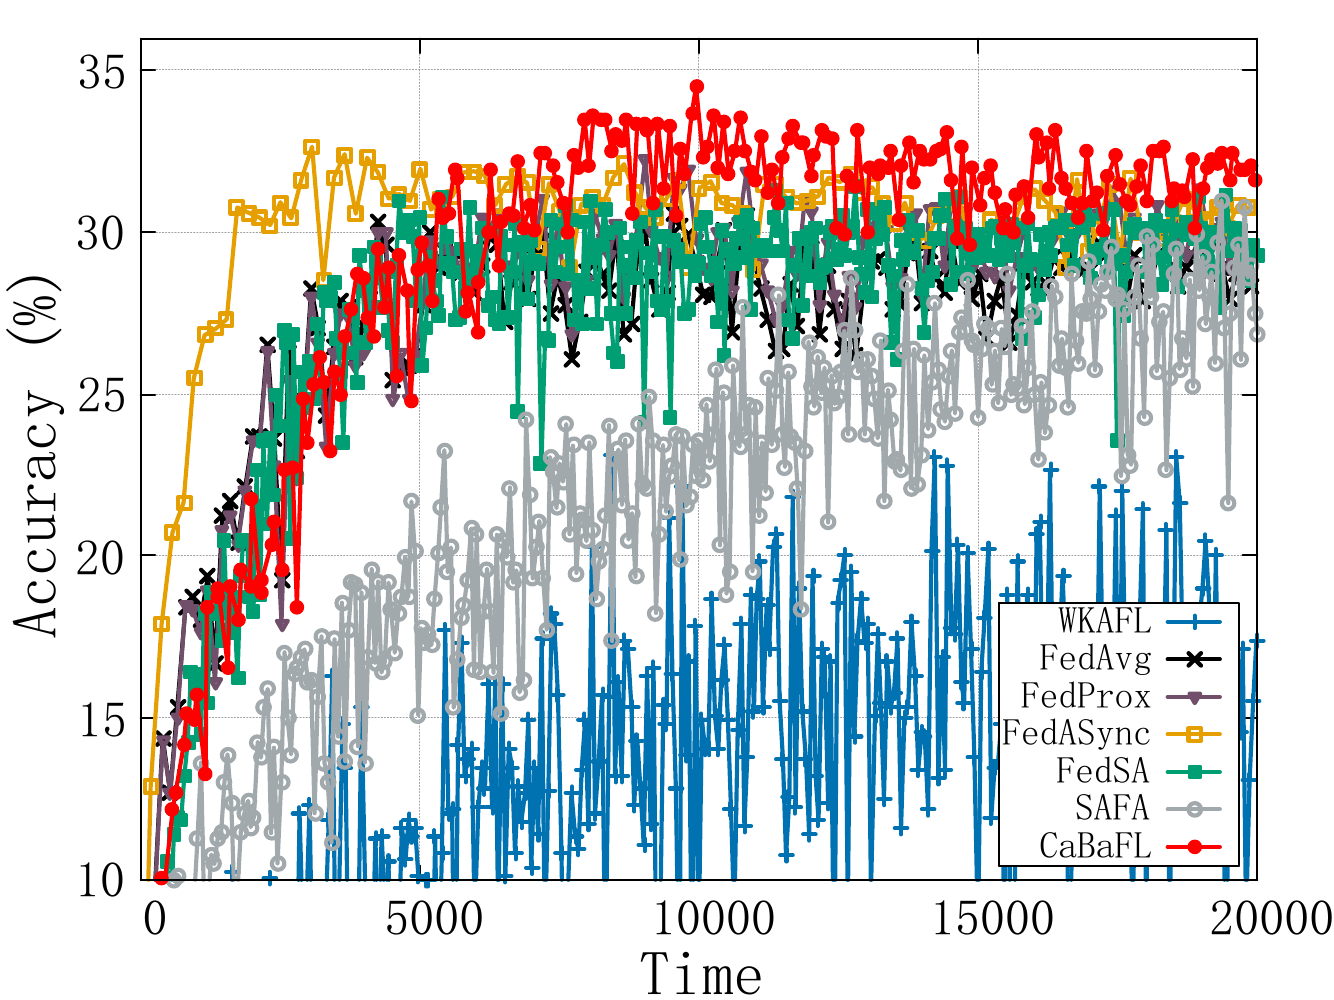}%
\label{}}
\hfil
\subfloat[$\beta = 0.5$]{\includegraphics[width=0.45\columnwidth]{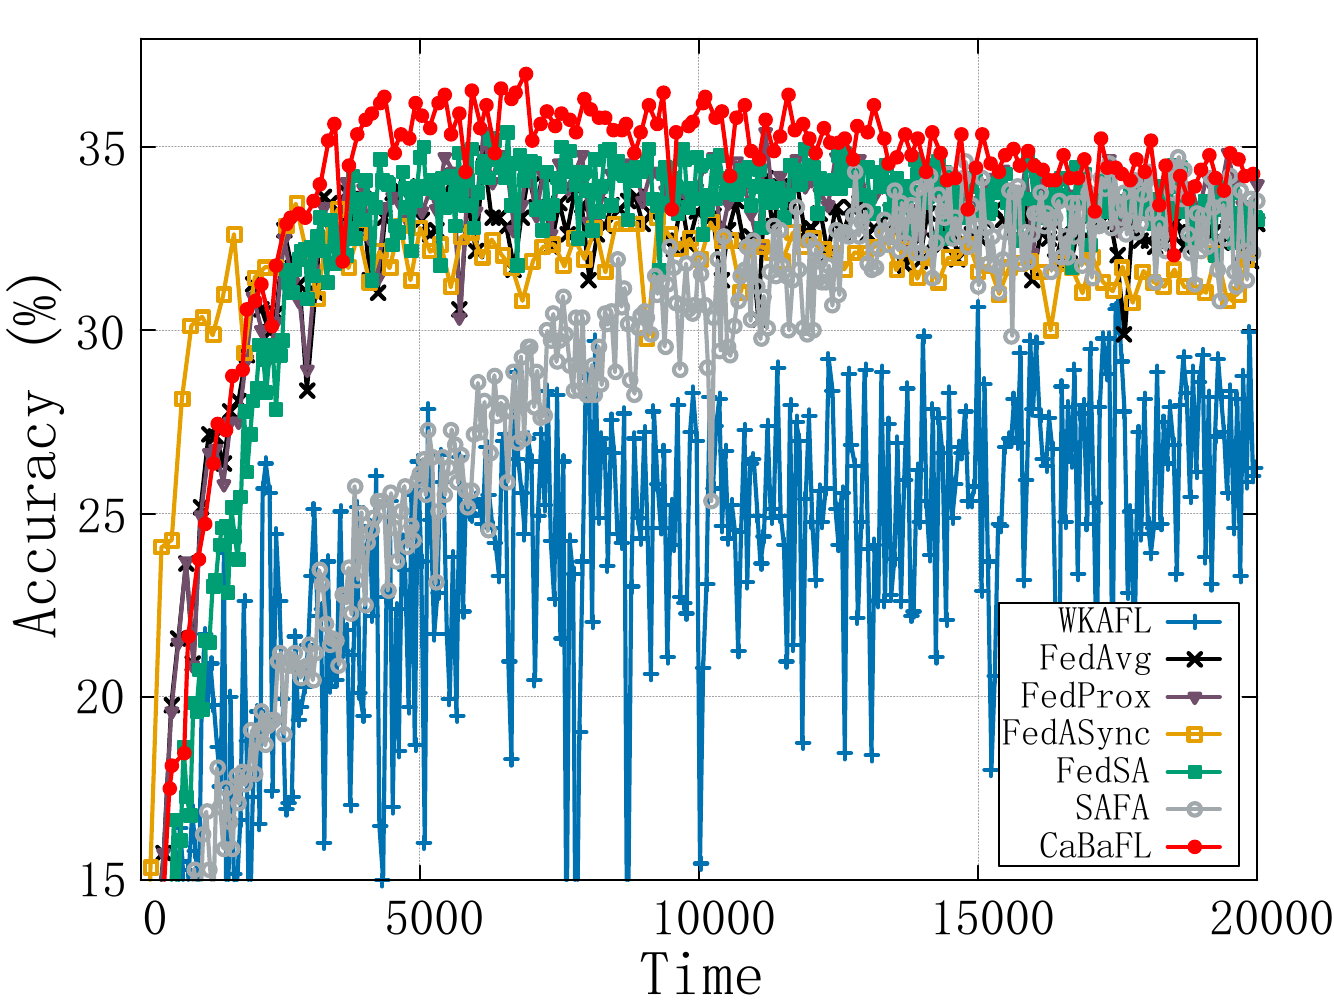}%
\label{}}
\hfil
\subfloat[$\beta = 1.0$]{\includegraphics[width=0.45\columnwidth]{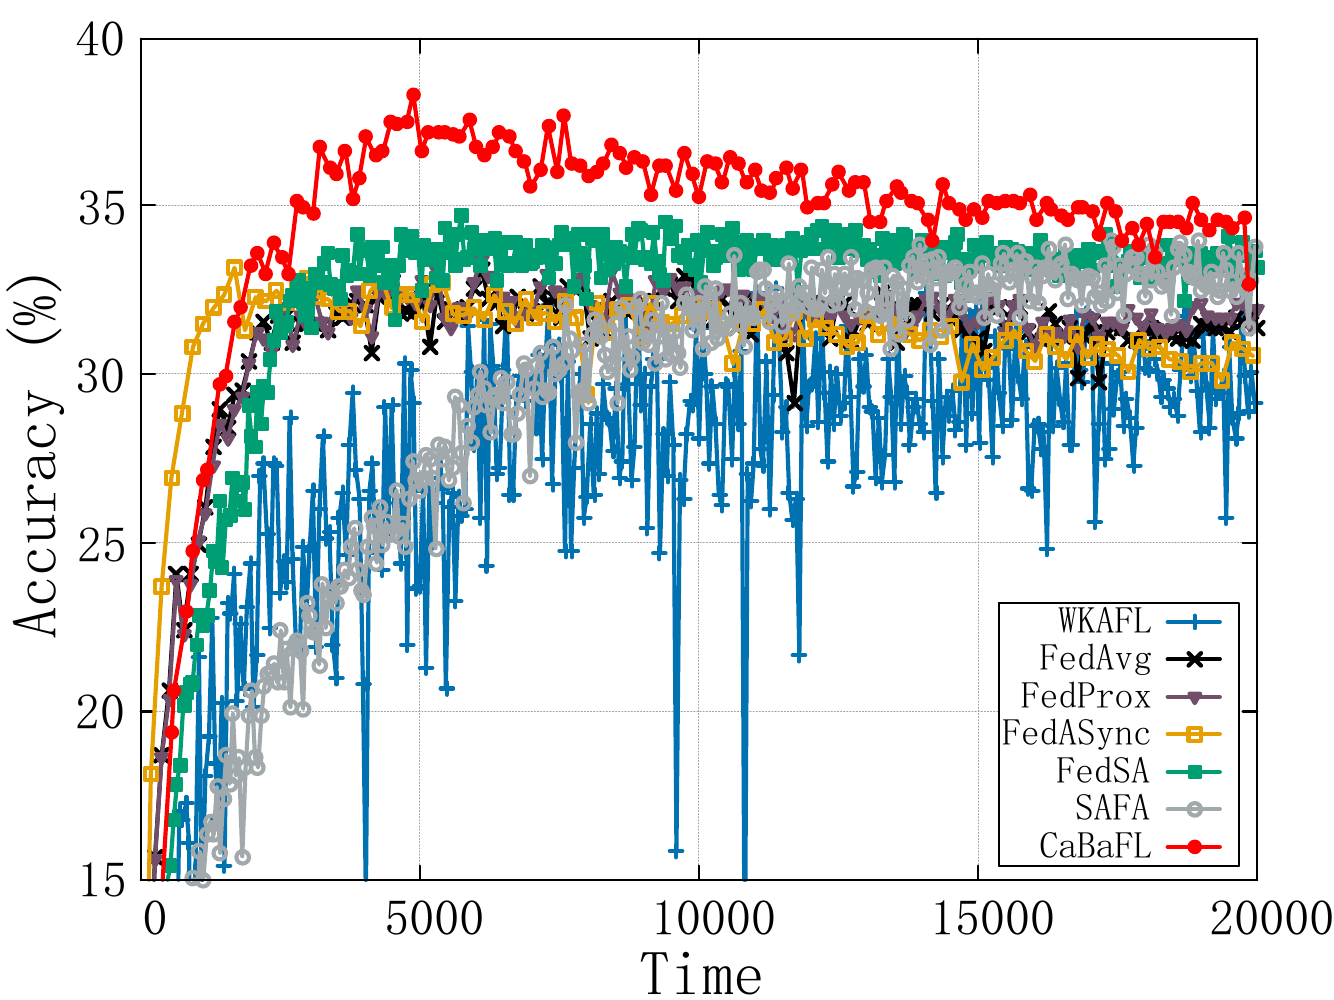}%
\label{}}
\hfil
\subfloat[IID]{\includegraphics[width=0.45\columnwidth]{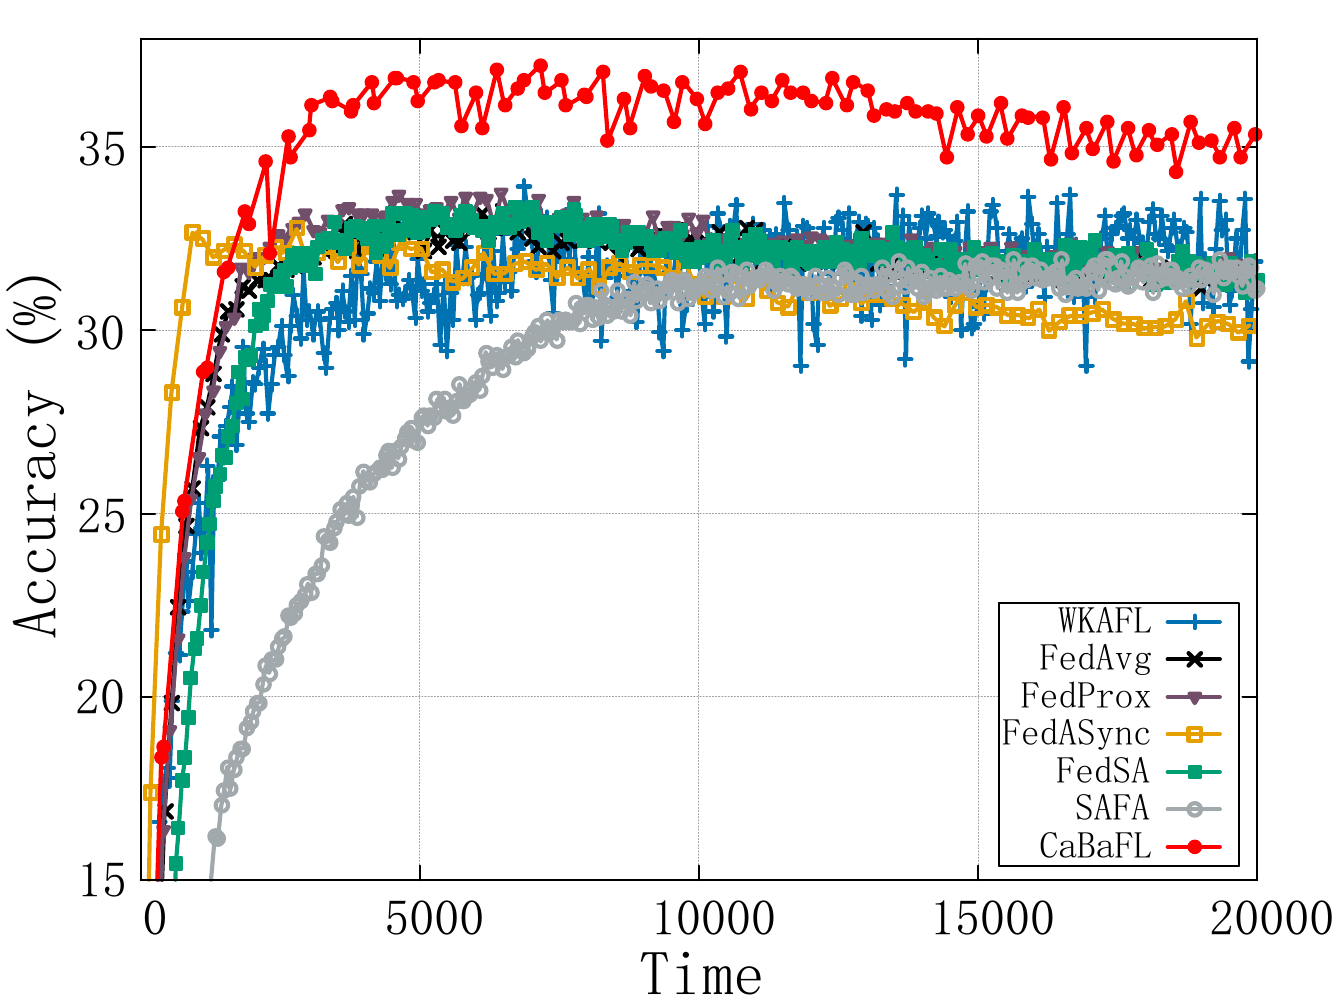}%
\label{}}
\caption{Learning curves of CaBaFL and all the baseline methods on CIFAR-100 and CNN.}
\label{end}
\end{figure}

\begin{figure}[h]
\centering
\footnotesize
\subfloat[$\beta = 0.1$]{\includegraphics[width=0.45\columnwidth]{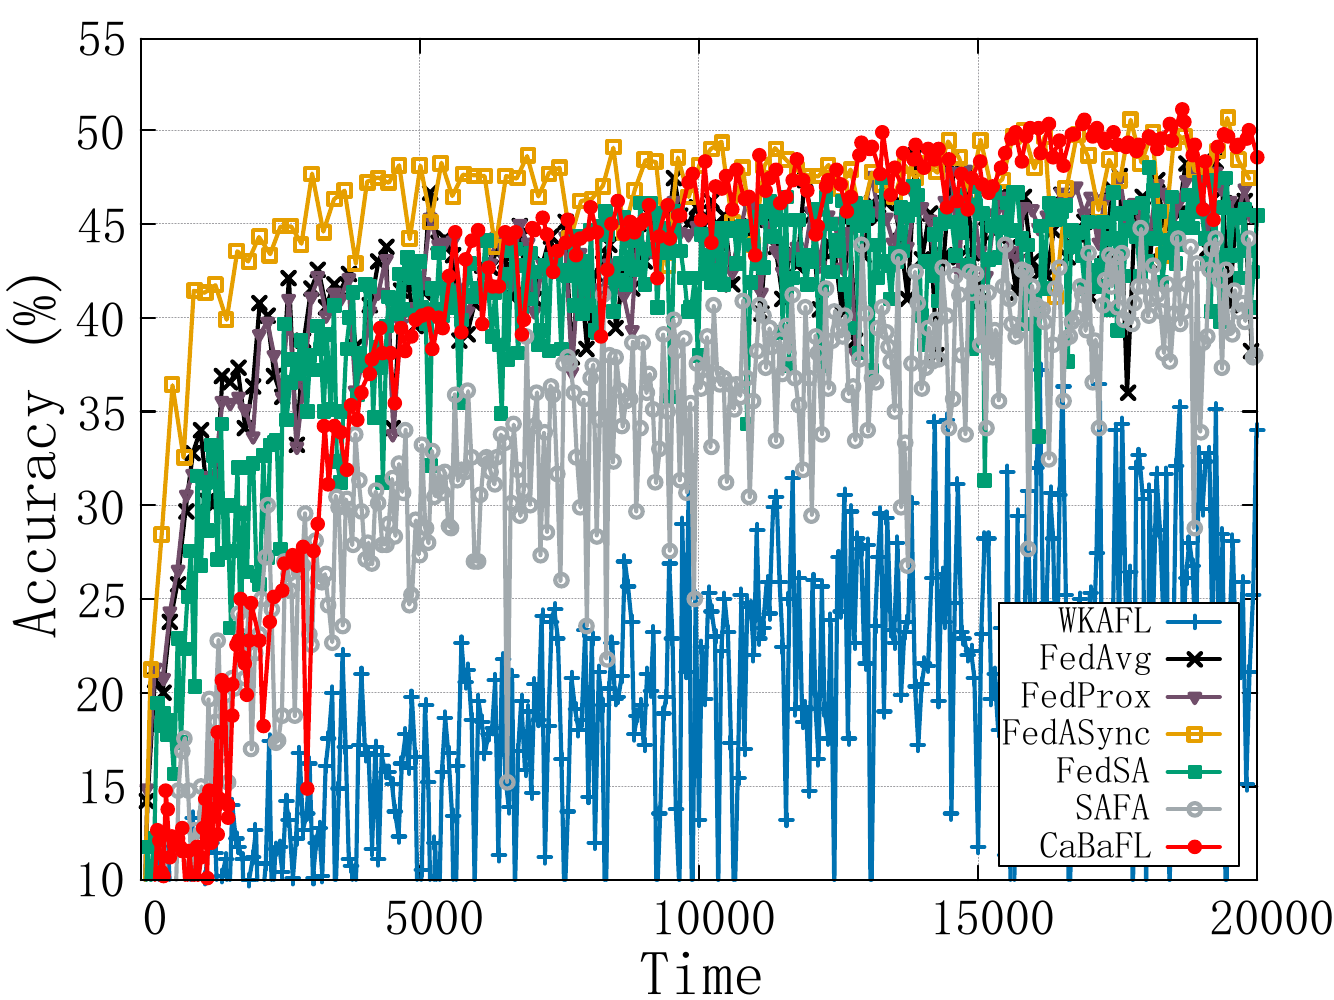}%
\label{}}
\hfil
\subfloat[$\beta = 0.5$]{\includegraphics[width=0.45\columnwidth]{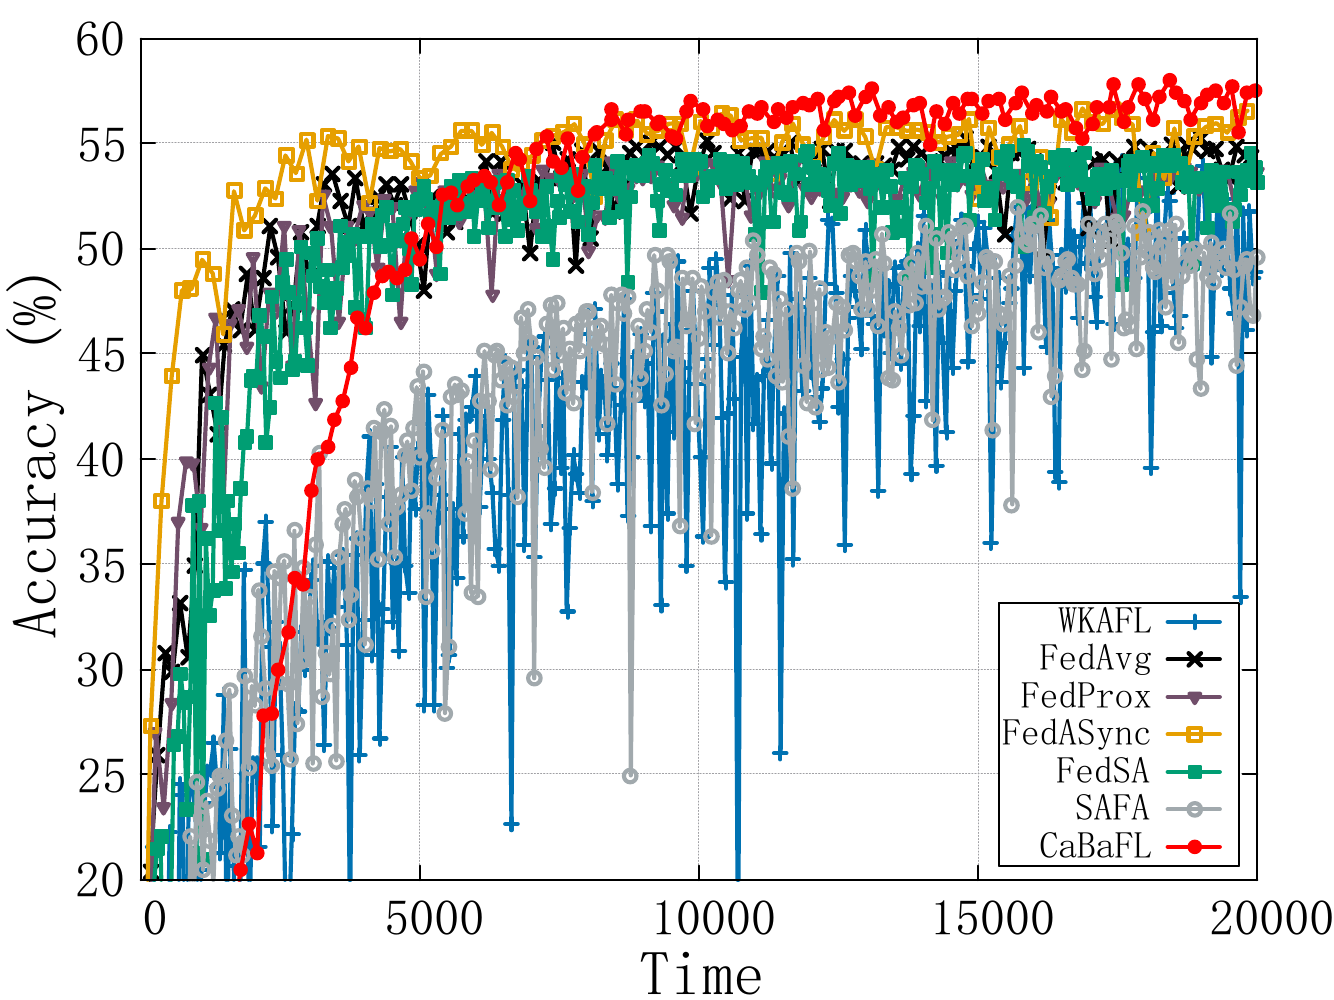}%
\label{}}
\hfil
\subfloat[$\beta = 1.0$]{\includegraphics[width=0.45\columnwidth]{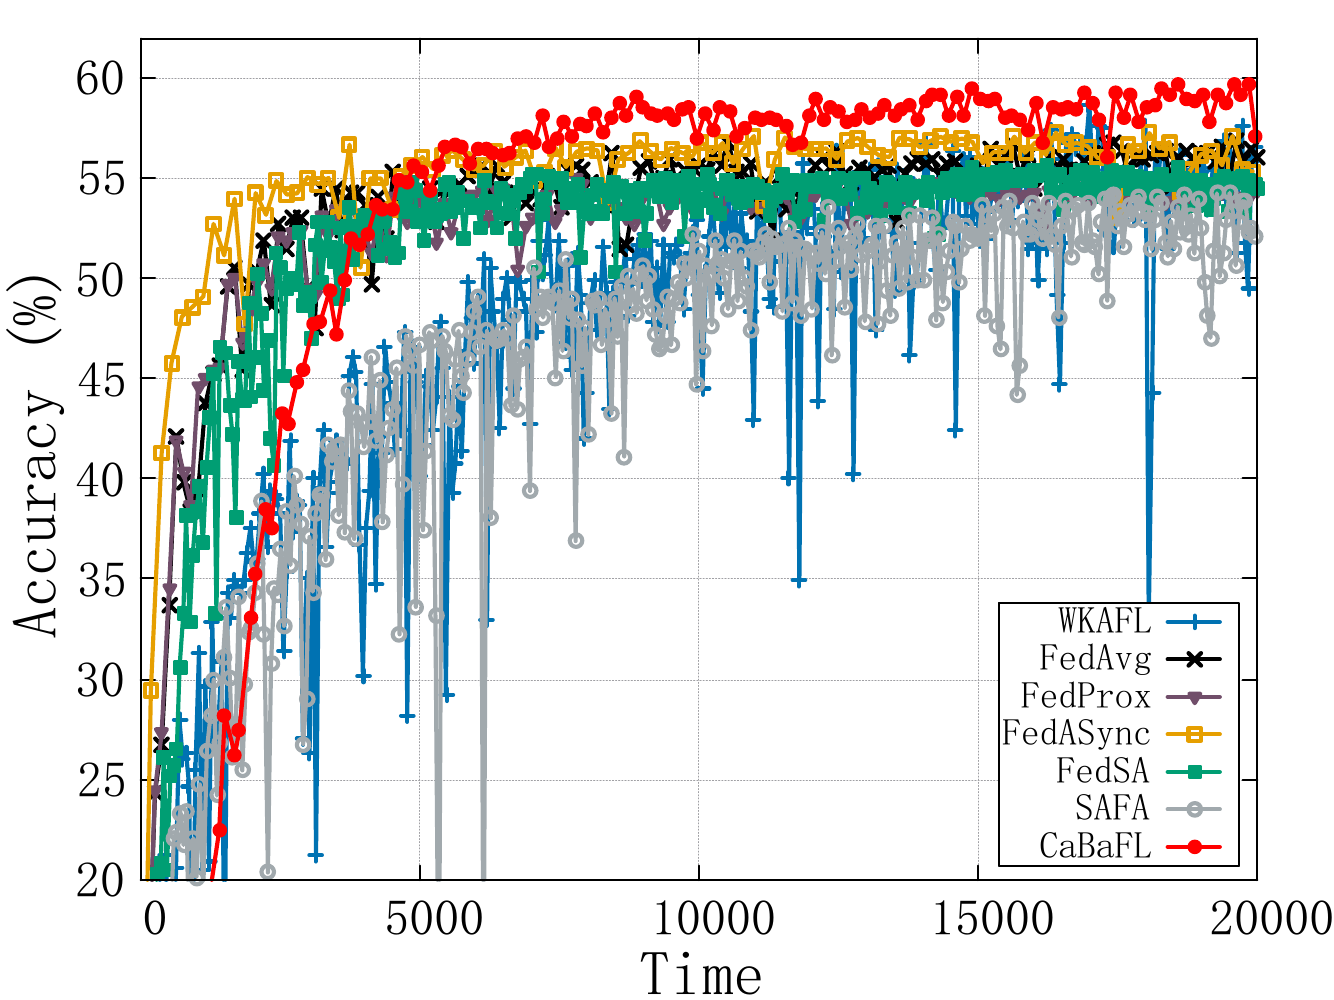}%
\label{}}
\hfil
\subfloat[IID]{\includegraphics[width=0.45\columnwidth]{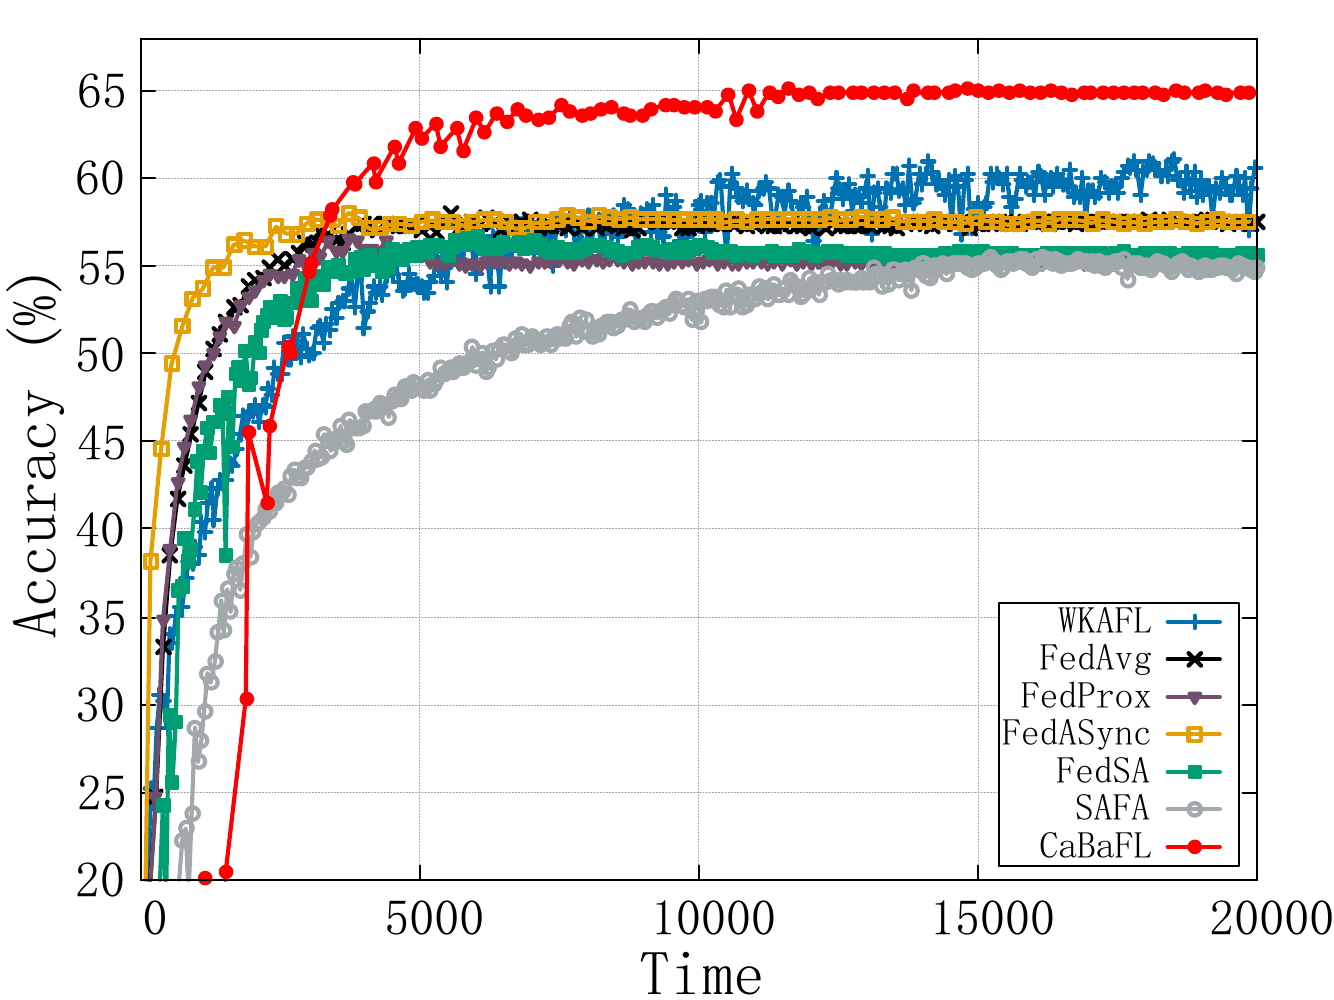}%
\label{}}
\caption{Learning curves of CaBaFL and all the baseline methods on CIFAR-100 and VGG-16.}
\end{figure}

\begin{figure}[h]
\centering
\footnotesize
\subfloat[ResNet-18]{\includegraphics[width=0.45\columnwidth]{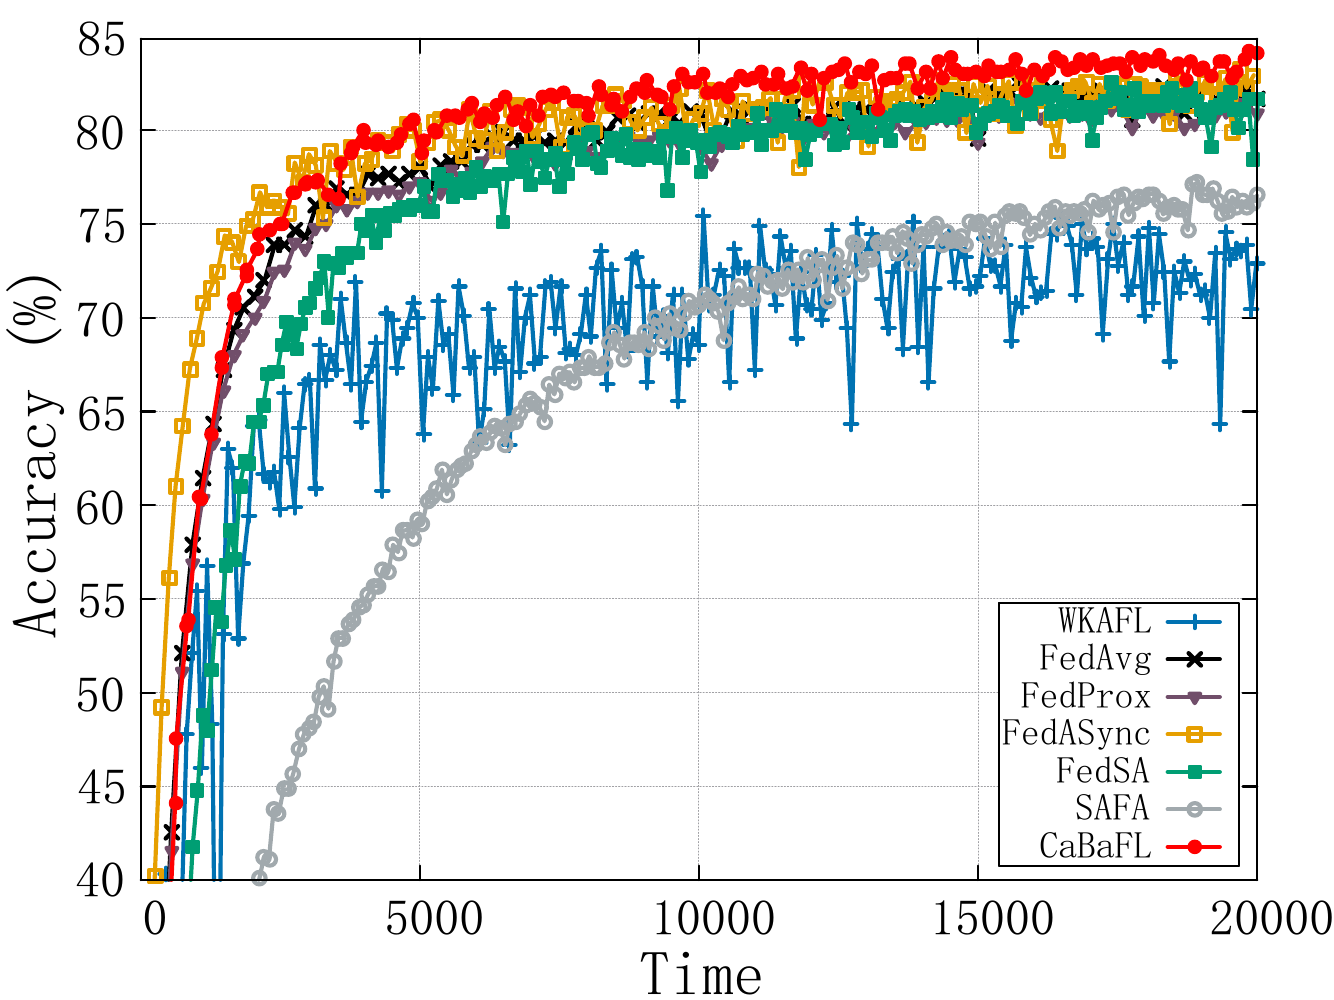}%
\label{}}
\hfil
\subfloat[CNN]{\includegraphics[width=0.45\columnwidth]{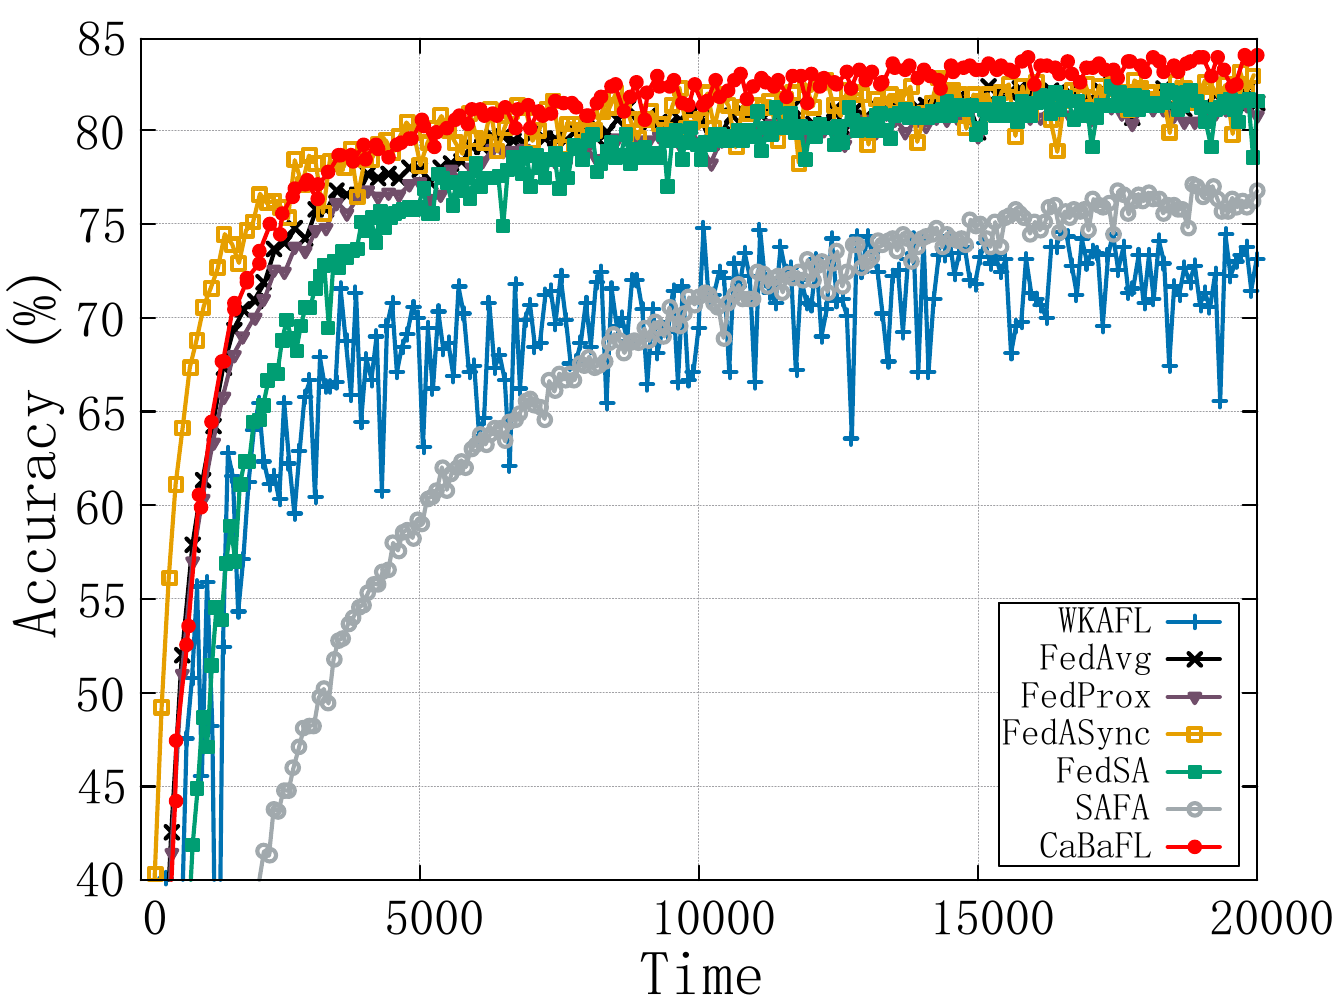}%
\label{}}
\hfil
\subfloat[VGG-16]{\includegraphics[width=0.45\columnwidth]{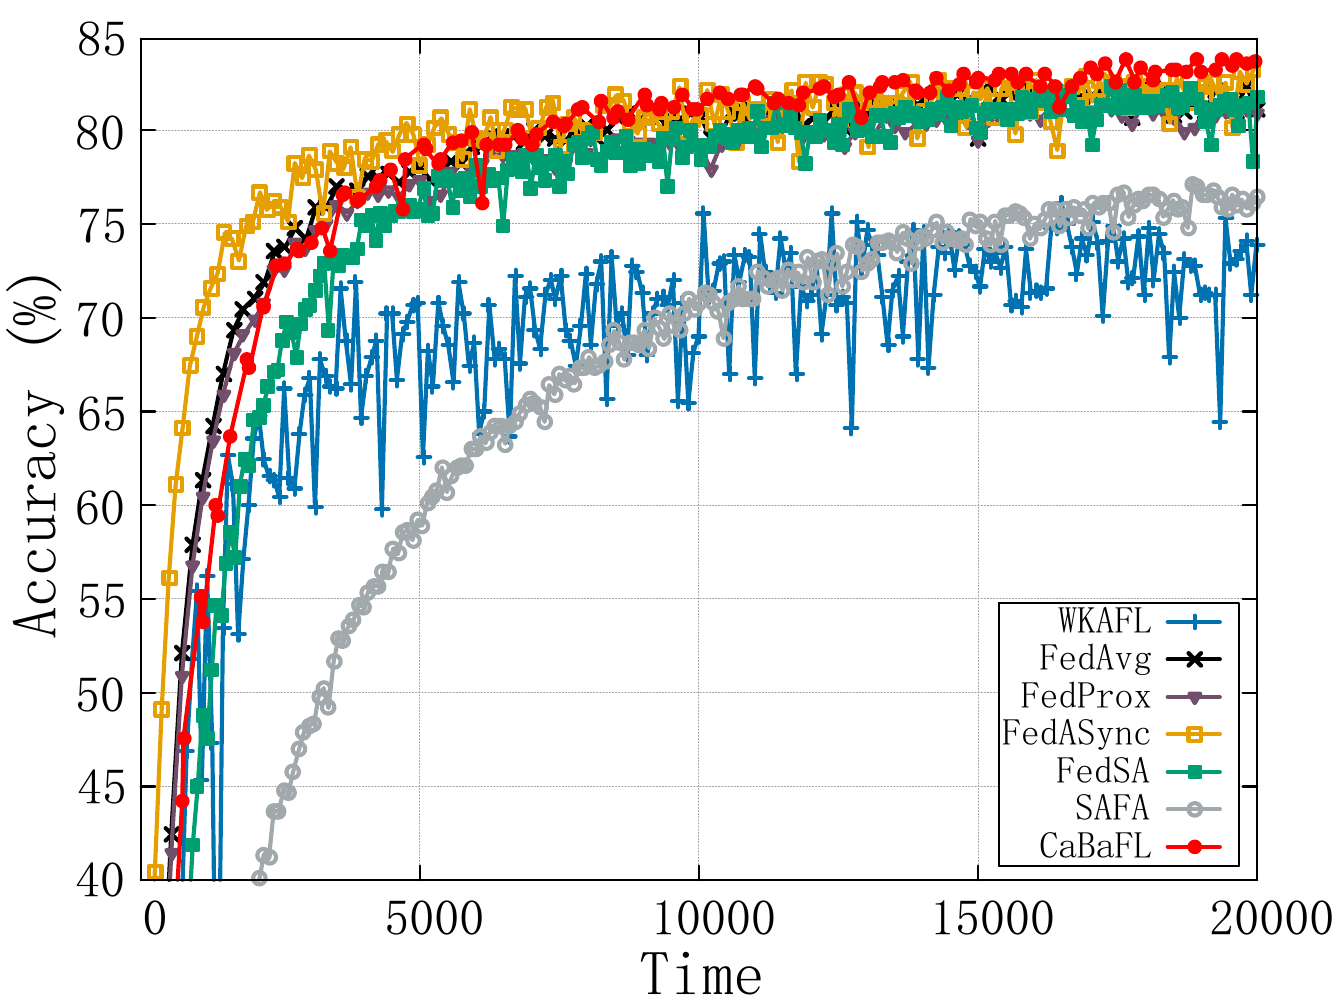}%
\label{}}
\caption{Learning curves of CaBaFL and all the baseline methods on FEMNIST with ResNet-18, CNN, and VGG-16.}
\end{figure}

\subsection{Discussion}
% \subsubsection{Adaptive Training Times}
% From Figure \ref{cifar10_vgg} (a) we can find that CaBaFL has a slower accuracy improvement in the early training period when using the VGG-16 model and $\beta=0.1$. This may be caused by too many model training times. To further investigate the impact of model training times $k$, we set up five different training times, respectively 4, 8, 10, 12, and 14, and conducted experiments using VGG-16 on CIFAR-10 with Dirichlet distribution where $\beta=0.1$. Figure \ref{fig:appendix_diff_k} exhibits the experiment result. We can find that although a larger $k$ will lead to slower accuracy improvement in the early stage of training, it can improve the stability and accuracy of training in the later stage of training. Therefore we may combine the advantages of larger $k$ and smaller $k$ by dynamically adjusting $k$. Currently, CaBaFL lacks a method that can adaptively adjust the training times of the models. We key how to find the optimal training times $k$ for our future work.
% \begin{figure}[H]
%   \begin{center} 
% 		\includegraphics[width=0.33\textwidth]{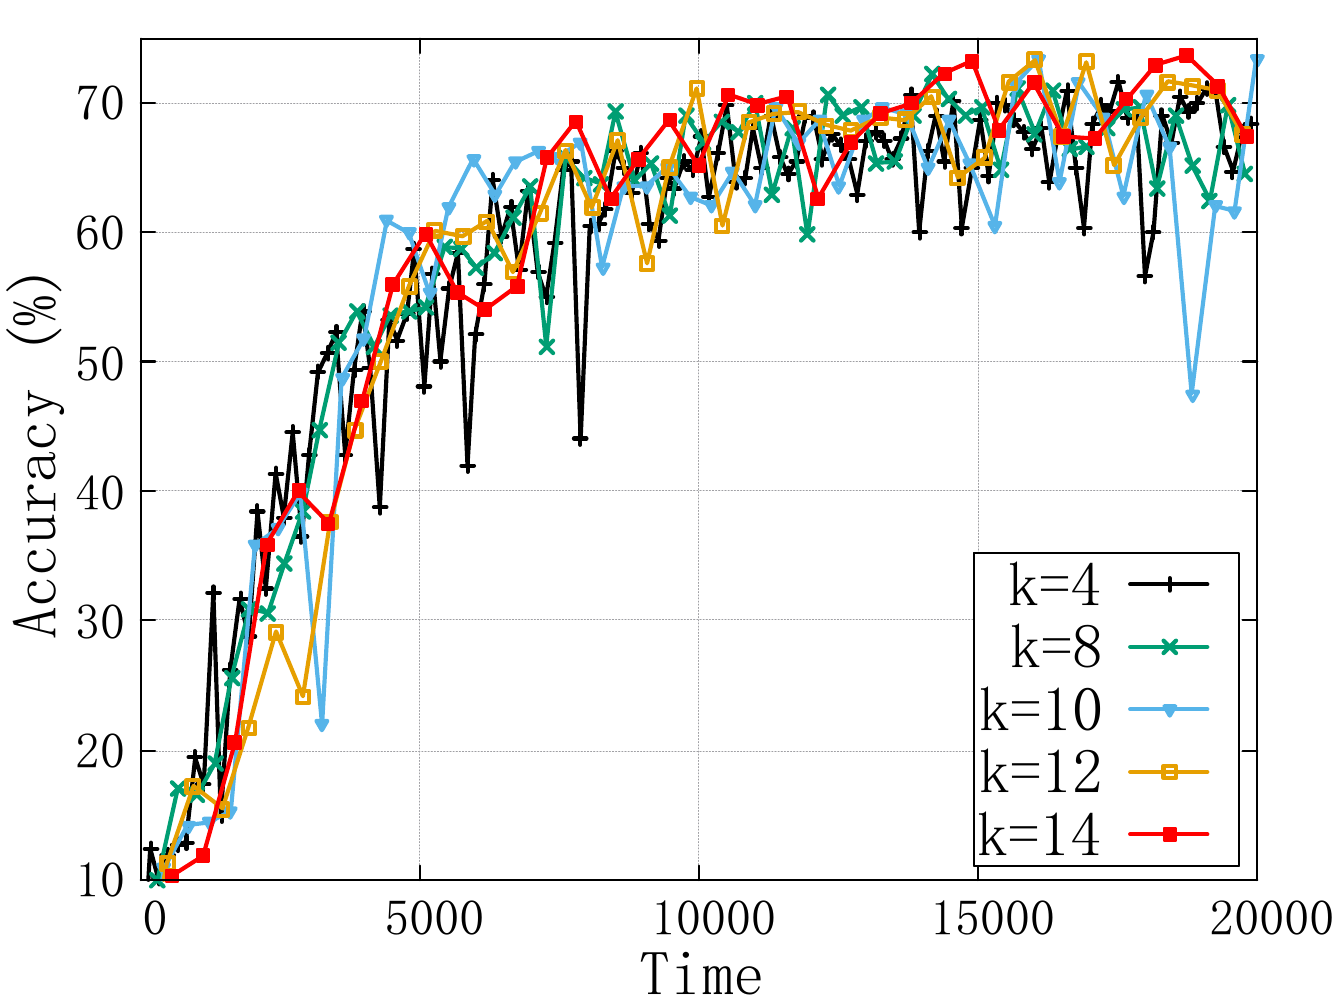}
% 		\caption{Impact of training times.}
% 		\label{fig:appendix_diff_k} 
% 	\end{center}
% \end{figure}

% \subsubsection{Overfitting}

% \subsection{Deployment of real-world scenarios}
